# Supplementary material for: Illuminating the Dark Sector: Searching for new interactions between dark matter and dark energy
Source: arXiv:2401.13814 source file (2024-01-24)
Supplement: Supplementary file 1 [file Appendix_A.tex]

%Main in MyThesis.tex

\chapter{Numerical Units}\label{sec:appa}
\setcounter{equation}{0}
\setcounter{figure}{0}

\subsection*{Natural Units}

\et{copy from thesis - reframe}

n order to make the calculations cleaner, it is universal practice in Cosmology to adopt the system of natural units where

\begin{equation}
c=\hbar=\epsilon_0=\mu_0=1.
\end{equation}

By doing so, the meaning of the equations becomes more straightforward and there is a more intuitive grasp on the order of magnitude of cosmological quantities.
By taking natural units we are collectively fixing the units of mass, length, time and charge relative to each other. This leaves only one unit free to fix them all which, by fundamental reasons, is usually taken to correspond to the dimensions in which energy is expressed, GeV, or equivalently:

\begin{equation}
\left[ E \right]=M,
\end{equation}

\noindent where the square brackets denote the dimensions of the quantity inside them and $M$ stands for dimensions of mass. This dimensional relation follows immediately from the relation between energy and mass, e.g. $E=mc^2$, with $c=1$. Also, this implies that time and length should have the same dimensions, which from $\hbar=1$ reads:

\begin{equation}
\left[ T \right]=M^{-1}
\end{equation}

\noindent and

\begin{equation}
\left[ L \right]=M^{-1}.
\end{equation}

For the energy density, defined as energy per unit volume, we find

\begin{equation}
\left[ \rho \right]=M^4.
\end{equation}

Following this, the dimensions of other useful cosmological variables can be derived

\begin{equation}
\left[ H \right]= \left[ \frac{\dot{a}}{a} \right] = M,
\end{equation}

\begin{equation}
\left[ \kappa \right]=\left[ \sqrt{8 \pi G} \right] = M^{-1},
\end{equation}

\noindent where $H$ is the Hubble factor and $\kappa$ is the scaled gravitational constant.

Since the action

\begin{equation}
S= \int d^4x \mathcal{L}
\end{equation} 

\noindent is a dimensionless quantity, we find for the Lagrangian density

\begin{equation}
\left[ \mathcal{L} \right] = M^{4}.
\end{equation}

The dimensions of a scalar field can be deduced by quantum field theory arguments. For quantum canonical fields the dimensions follow from the free-field Lagrangian density:

\begin{equation}
\mathcal{L}_{\rm free} \equiv \frac{1}{2} \partial_{\mu} \Phi \partial^{\mu} \Phi - \frac{1}{2} m^2 \Phi^2,
\end{equation}

 \noindent leading to
 
 \begin{equation}
 \left[ \Phi \right] = M.
 \end{equation}
 
In fact, because of the kinetic term given in terms of partial derivatives of the field, all bosonic fields in 4-dimensional spacetimes have canonical dimensions of mass.
 
Another example are the fermionic fields like the Dirac field $\psi (x)$ with free Lagrangian density given by

\begin{equation}
\mathcal{L}_{\rm free} \equiv \bar{\Psi} \left( i \gamma^{\mu} \partial_{\mu} - m \right) \Psi.
\end{equation}

This means that for the Dirac fields

 \begin{equation}
 \left[ \Psi \right] =  \left[ \bar{\Psi} \right]= M^{3/2}.
 \end{equation}
 
In fact, because of the presence of the kinetic term with two fields and one partial derivative, all types of fermionic fields in 4-dimensional spacetimes have canonical dimension mass$^{3/2}$.
 For non-canonical scalar fields the dimensions could become non-standard. For instance, the Lagrangian density for the tachyon field is defined as
 
 \begin{equation}
 \mathcal{L}_{\rm tach} \equiv - V(\phi) \sqrt{1+g^{\mu \nu} \partial_{\mu} \phi \partial_{\nu} \phi}.
 \end{equation}
 
 \noindent Since $V$ stands for the potential energy density associated to the field, 
 
 \begin{equation}
 \left[ V \right]= M^4,
 \end{equation}
 
 \noindent from where we conclude that the dimensions for the tachyon field are
 
 \begin{equation}
 \left[ \phi \right] = M^{-1}.
 \end{equation}

\subsection*{Background Units}

Internally, the code uses almost everywhere units of Mpc to some power.

Class computes the expansion rate from the Friedmann equation.

Unless otherwise specified in the input file, the units and the definition of the output quantities are written in comment lines at the top of each output file.

The units are inverse mega-parsecs for wavenumbers $k$ and for the Hubble rate, and mega-parsecs for conformal time, $\tau$:

\begin{itemize}
\item $[H]=[k]={\rm Mpc}^{-1},\ [\tau] = {\rm Mpc}$.
\end{itemize}

For background densities $\rho_i$ and pressure $p_i$, more unusual units are used. The goal is to be able to write the Friedmann equation as:

\begin{equation}
H=\left(\sum_{i=0}^{N} {\rm rho}\_i \right)^{1/2}.
\end{equation}

Hence, everywhere in the code, the density ${\rm rho}\_i$ stands for $[8 \pi G {\rm rho}\_i/3]$ (same for the pressure ${\rm p}\_i$). Densities are all expressed in units of $3c^2/(8 \pi G)$, i.e.:

\begin{equation}
\rho_{\rm class} = \frac{8 \pi G}{3 c^2} \rho_{\rm physical}.
\end{equation}

In the output file all densities are multiplied by $8 \pi G/3$.

Densities are in units of in of inverse squared mega-parsecs while all distances are in mega-parsec:

\begin{itemize}
\item $[{\rm rho}\_i]=[{\rm p}\_i]={\rm Mpc}^{-2},\ [d] = {\rm Mpc}$.
\end{itemize}

In Class conventions the critical density is just H$_0$.

In this scenario $h$ is dimensionless and

\begin{itemize}
\item $[{\rm H}_0/c]={\rm Mpc},\ {\rm with}\  {\rm H}_0/c=h/2997.9=h*10^5/c$.
\end{itemize}

This means that:

\begin{equation}
{\rm H}_0={{\rm H}_0}_{\rm planck}*10^{3}/c,\ h={\rm H}_0/100,\ {\rm H}_0=h*10^5/c.
\end{equation} 

The Planck mass and the reduced Planck mass are expressed in units of inverse mega-parsec and mega-parsec, respectively:

\begin{itemize}
\item $[k]=[\sqrt{8 \pi G}]={\rm Mpc},\ [{\rm M}_{\rm pl}]=[k^{-1}]={\rm Mpc}^{-1}$.
\end{itemize}

\subsection*{Units of scalar field related quantities}

The field is given in units of the reduced Planck mass $(8 \pi G)^{-1/2}$.

The potential is given in units of M$_{\rm Pl}^2/{\rm Mpc}^2$.

Units summarised:

\begin{itemize}
\item $\left[ \td{\phi} \right]=\left[ \frac{\phi}{{\rm M}_{\rm Pl}} \right] = {\rm dimensionless}$.

\item $[V]=\left[V_0 {\rm M}_{\rm Pl}^4 \td{\phi}^2\right] = {\rm M}_{\rm Pl}^{2} {\rm Mpc}^{-2} \Leftrightarrow [V_0] = {\rm Mpc}^{-2} * {\rm M}_{\rm Pl}^{-2}$.

\item $[h]=\left[h_0 {\rm M}_{\rm Pl}^{-4} \td{\phi}^{-4}\right] = {\rm Mpc}^{2}  {\rm M}_{\rm Pl}^{-2} \Leftrightarrow [h_0] = {\rm Mpc}^{2} * {\rm M}_{\rm Pl}^{2}.$
\end{itemize}

This means that $\rho_{\rm class}$ is defined as:

\begin{equation}
\rho_{\rm class} = \frac{8 \pi G}{3 c^2} \rho_{\rm physical} = \frac{1}{{3 {\rm M}_{\rm Pl}}}\rho_{\rm physical} =\frac{1}{{3 {\rm M}_{\rm Pl}}}\left[\frac{1}{2a^2} \phi'^2 + V(\phi) \right] =\frac{1}{3}\left[\frac{1}{2a^2} \td{\phi}^2 + V(\td{\phi} ) \right],
\end{equation}

\noindent and has the proper dimensions of Mpc$^{-2}$.

Fix the initial values of phi and phi' set directly in the radiation attractor. This fixes the units in terms of ${\rm rho}\_{\rm rad}$.

\subsection*{Conversion of units defined in the code}

In the code the following variables are defined:
\begin{itemize}
\item Conversion factor from meter to mega-parsec: $\_{\rm Mpc}\_{\rm over}\_{m}\_ = 3.085677581282e22$

\item c in ms$^{-1}$: $\_c\_ = 2.99792458e8$

\item Newton constant in m$^3$kg$^{-1}$s$^{-2}$: $\_G\_ = 6.67428e-11$

\item 1 eV expressed in J: $\_eV\_ = 1.602176487e-19$

\end{itemize}

We want to use these conversions to define the potential in units of ${\rm Mpc}^{-2}$:
 
 \begin{itemize}
\item ${\rm GeV}$ to ${\rm cm}^{-1}$: $1\ {\rm GeV} = 5.06765 \times 10^{13}\ {\rm cm}^{-1}$

\item ${\rm M_{Pl}}$ to ${\rm GeV}$: $1\ {\rm M_{Pl}} = 2.435 \times 10^{18}\ {\rm GeV}$

\item ${\rm M_{Pl}}$ to ${\rm cm}^{-1}$: $1\ {\rm M_{Pl}} = 1.23397 \times 10^{32}\ {\rm cm}^{-1}$

\item ${\rm M_{Pl}}$ to ${\rm Mpc}^{-1}$: $1\ {\rm M_{Pl}} = 3.80767 \times 10^{56}\ {\rm Mpc}^{-1}$
\end{itemize}

This means that ${\rm M_{Pl}}^2 = 1.44983 \times 10^{113}\ {\rm Mpc}^{-2}$ and this conversion factor should be used in the definition of $V_0$.

\et{include also tachyons?}

\subsection*{References}\label{ref}

https://usermanual.wiki/Pdf/CLASSMANUAL.1775036913/view
