# Supplementary material for: Illuminating the Dark Sector: Searching for new interactions between dark matter and dark energy
Source: arXiv:2401.13814 source file (2024-01-24)
Supplement: Supplementary file 2 [file Appendix_C.tex]

\chapter{Health of Disformal Transformations of the Metric} \label{chap:appdisf}
\setcounter{equation}{0}
\setcounter{figure}{0}

We can formally define the "health" of a metric transformation by a set of conditions: it must preserve Lorentzian signature, be causal, and remain invertible with a non-zero volume element. All of these properties directly impose constraints on the two free functions $\Omega$ and $\Gamma$, which are summarised below:

\begin{enumerate}
    \item \textit{Causality}: In contrast with the conformal case, the causal structure of the spacetime is no longer preserved and the light cones are affected by the transformation
\begin{equation}
    \odif{s}^2 \mapsto \odif{\td{s}}^2 = \Omega^2  \dd g_{\mu \nu} x^{\mu} \dd x^{\nu} + \Gamma \left( \partial_{\mu} \phi\, \dd x^{\mu} \right)^2 = \Omega^2 \odif{s}^2 + \Gamma \left( \partial_{\mu} \phi\, \dd x^{\mu} \right)^2 \mathcomma
\end{equation}
meaning that the light cones of $\bar{g}$ become wider or narrower depending on the sign of $\Gamma$, than those of the metric $g$. This might lead one to consider that particles moving along one of the transformed metrics could exhibit superluminal or acausal behavior. However, such considerations involve the \textit{a priori} choice of a reference chronology, while in geometric terms, both metrics are on equal footing and it could be misleading to pick one of them to define causality.
Moreover, the requirement of the invariance of the squared line element and the fact that physical particles satisfy $\odif{s}^2 < 0$ are sufficient to ensure causal behaviour. This objection has been thoroughly discussed in \cite{Bruneton:2006gf}.

\item  \textit{Lorentz signature}: A feature that must also still hold is the Lorentzian signature of the metric. In the FLRW scenario this means that
\begin{equation}
    g_{00} < 0 \mapsto \td{g}_{00} = \Omega^2 g_{00} + \Gamma \partial_0 \phi \partial_0 \phi < 0 \mathcomma
\end{equation}
which must be verified for all values of the field and its derivatives. Keeping in mind that the disformal function can vanish for particular scalar field values we must guarantee that $\Omega^2>0$, which had already been considered. Assuming that $\partial_{\mu} \phi = \left( \dot{\phi}, 0,0,0 \right)$, this condition can be simplified by multiplying both sides by $g^{00}$, resulting in 
\begin{equation}
    \Omega^2 + \Gamma g^{00} \dot{\phi}^2 = \Omega^2 - 2 \Gamma X >0 \mathcomma
    \label{eq:lor}
\end{equation}
which is the condition imposed by the Lorentz signature preservation. 

\item \textit{Non-singular inverse metric}: The inverse metric is defined by ensuring that $g^{\mu \nu} g_{\mu \sigma} = \td{g}^{\mu \nu} \td{g}_{\mu \sigma} = \delta^{\mu}_{\sigma}$, which results in
\begin{equation}
    \td{g}^{\mu \nu} = \frac{1}{\Omega^2 (\phi,X)} g^{\mu \nu} - \frac{\Gamma (\phi,X)}{\Omega^2 (\phi,X)} \frac{\covd^{\mu} \phi \covd^{\nu} \phi}{\Omega^2 (\phi,X) -2 \Gamma (\phi,X) X} \mathperiod
\end{equation}
In order for $\td{g}^{\mu \nu}$ to be non-singular then the terms in the numerators must never vanish and the constraint in \cref{eq:lor} becomes
\begin{equation}
    \Omega^2 \neq 0,\ \ \ \Omega^2 - 2 \Gamma X > 0 \mathperiod
    \label{eq:nsinv}
\end{equation}

\item \textit{Non-singular volume element}: The volume element is given by
\begin{equation}
    \sqrt{- \td{g}} = \Omega^4 \sqrt{ 1 - 2 X \frac{\Gamma }{\Omega^2}} \sqrt{-g} \mathcomma
\end{equation}
and is already guaranteed to be non-singular if the previous conditions hold.

\end{enumerate}

This all comes together by requiring the conditions in \cref{eq:nsinv}.
