# Supplementary material for: Illuminating the Dark Sector: Searching for new interactions between dark matter and dark energy
Source: arXiv:2401.13814 source file (2024-01-24)
Supplement: Supplementary file 3 [file Appendix_D.tex]

\chapter{Disformally Coupled Quintessence} \label{app:disformal}
\setcounter{equation}{0}
\setcounter{figure}{0}

 For the sake of comparison we present here the equations for a disformally coupled dark sector. \et{rewrite}

% Clarifying our model - detailing the action
To provide a lucid account of what we understand by conformal and disformal transformations in the realm of dark matter geometry, let us delineate the action of the theoretical framework under consideration:
\begin{equation}
\label{eq:definedAction}
\mathcal{S} = \int d^4x \sqrt{-g} \left\{ \frac{\mathcal{R}(g)}{2\kappa} + \mathcal{L}_{\text{(SM)}} + \mathcal{L}_{\text{(DE)}} \right\} + \int d^4x \sqrt{-\tilde{g}} \tilde{\mathcal{L}}_{\text{(DM)}},
\end{equation}
where SM represents the observable sector (i.e., particles in the standard model) and dark energy, $\mathcal{L}_{\text{(DE)}}$, is characterized by a quintessence field:
\begin{equation}
\mathcal{L}_{\text{(DE)}} = -\frac{1}{2} \nabla^{\alpha} \phi \nabla_{\alpha} \phi - V(\phi).
\end{equation}
The Lagrangian describing the dark matter sector,
\begin{equation}
\tilde{\mathcal{L}}_{\text{(DM)}} = \tilde{\mathcal{L}}_{\text{(DM)}}(\tilde{g}_{\alpha\beta};\varphi),
\end{equation}
is a function of the metric
\begin{equation}
\label{eq:detailedDismetric}
\tilde{g}_{\mu\nu} = C(\phi)g_{\mu\nu} + D(\phi)\phi,_{\mu} \phi,_{\nu}.
\end{equation}
The functions $V$, $C$, and $D$ encapsulate the remaining degrees of freedom in our theory, to be further outlined in ensuing sections. `Conformal factor' and `disformal factor' are the terms by which $C$ and $D$ are commonly known. We observe that the geodesics followed by dark matter particles are dictated by $\tilde{g}_{\mu\nu}$, and various properties of these particles, such as their mass, are now influenced by the dark energy field. We omit the possibility that $C$ and $D$ may depend on the derivatives of $\phi$, for the sake of simplicity in this work.

% Describing the scope of the theory
The articulated theory serves as a mathematical instantiation of generalized gravitational interactions in the dark sector. It accommodates a vast, albeit not exhaustive, array of deviations from general relativity, which now represents a specific point in function space: $C=1$ and $D=0$. The case with $D=0$ but $C\neq 1$ has garnered much discussion, and the role of the disformal term has recently begun to receive attention. We will focus on models with $C\neq 1$ and $D\neq 0$, contrasting them to models with purely conformal terms. Notably, we will numerically investigate the interplay between the two types and find that one can effectively suppress the other.

% Structuring the paper
The remainder of the paper is organized as follows: The subsequent section delves into the evolution of the background system and enumerates the various choices for the forms and parameters of the free functions ($V$, $C$, and $D$) that are consistently applied throughout our study. In Section 3, we shift our focus towards the cosmological perturbations in the presence of both disformal and conformal couplings and calculate matter and angular power spectra for different scenarios. Our conclusions are encapsulated in Section 4. All computational results, comprising background simulations and both types of power spectra, are generated using a modified version of the publicly available Boltzmann code CLASS \cite{Blas:2011rf}. Throughout the manuscript, we will stress the discernability of coupling types: can a purely disformal phenomenon actually be 'observed'?

\section{Cosmological Fundamentals}
\label{sec:background}

This section is divided into various subsections. We first present the fundamental equations governing the background, followed by an in-depth exploration of the background dynamics. Next, we delve into the effective coupling affecting dark matter as well as the effective equation of state governing the dark energy scalar field.

\subsection{Dynamics Equations}
The background spacetime adopts the canonical Friedmann--Robertson--Walker (FRW) metric, a solution to Einstein's field equations for the metric \( g_{\mu\nu} \), featuring flat spatial hypersurfaces:
\begin{equation}
\label{eq:CanonicalFRW}
ds^2 = g_{\mu\nu}dx^{\mu}dx^{\nu} = a^2(\tau)[-d\tau^2 + \delta_{ij}dx^idx^j].
\end{equation}
Here, \(\tau\) denotes the conformal time, and \(a(\tau)\) is the scale factor. Throughout the paper, dots signify derivatives with respect to \(\tau\).
The disformal metric, which dark matter particles perceive, is articulated by \cref{eq:detailedDismetric,eq:CanonicalFRW} as:
\begin{equation}
\label{eq:DisformalLine}
d\tilde{s}^2 = \tilde{g}_{\mu\nu}dx^{\mu}dx^{\nu} = Ca^2(\tau)[- \gamma^2 d\tau^2 + \delta_{ij}dx^idx^j],
\end{equation}
where we introduce a disformal scalar \(\gamma\) via:
\begin{equation}
\label{eq:DisformalScalar}
\gamma := \sqrt{1 + \frac{D}{C}g^{\mu\nu}\phi,_{\mu}\phi,_{\nu}}.
\end{equation}
The scalar field's background value is a function solely of \(\tau\).

% Visible sector specifics
We make the assumption that neutrinos are massless in our study. Consequently, the theory's different sectors are defined by a massless relativistic component \( r \), a baryonic component \( b \), a dark matter component \( c \), and the scalar field \( \phi \). Both the relativistic and baryonic species are postulated to be uncoupled from the scalar, hence their energy densities evolve according to standard conservation equations:
\begin{subequations}
\label{eq:StandardConservation}
\begin{align}
\label{eq:StandardConservation:r}
\dot{\rho}_{\rm r} + 3{\mathcal H} (\rho_{\rm r} + P_{\rm r}) &= 0,
\\
\label{eq:StandardConservation:b}
\dot{\rho}_{\rm b} + 3{\mathcal H} \rho_{\rm b} &= 0,
\end{align}
\end{subequations}
where \( P_{\rm r} = \rho_{\rm r}/3 \).

% Dark energy
The scalar field adheres to the Klein-Gordon equation and is coupled to dark matter through a coupling function \( Q \):
\begin{equation}
\label{eq:KleinGordonBG}
\ddot \phi + 2 {\cal H} \dot\phi + a^2 \frac{dV}{d\phi} = a^2 Q,
\end{equation}
with \( Q \)'s background form given by:
\begin{equation}
\label{eq:BackgroundQ}
Q = \ldots
\end{equation}

% Dark matter
Non-conservation in the energy--momentum tensor of dark energy leads to a corresponding non-conservation in dark matter. Thus, energy loss in one sector must correspond to an energy gain in the other, leading to the following for the cold dark matter species \( c \):
\begin{equation}
\label{eq:NonConservation}
\dot\rho_{\rm c} + 3 {\cal H} \rho_{\rm c} = - Q \dot \phi.
\end{equation}

% Gravitational dynamics
Finally, the Friedmann equation arising from Einstein's field equations is presented in its conventional form as:
\begin{equation}
\label{eq:CanonicalFriedmann}
{\cal H}^2 = \frac{8\pi Ga^2}{3} \left( \rho_{\rm r} + \rho_{\rm b} + \rho_{\rm c} + \rho_{\rm de} \right),
\end{equation}
where \( {\cal H} = \dot a/a \) and \( \rho_{\rm de} = \dot\phi^2/2a^2 + V(\phi) \).

\subsection{Examination of Field Dynamics}
The interaction between dark energy and dark matter in the preceding equations establishes an intriguing framework. The effective potential for the dark energy field is modulated by the coupling and is generally a function of $\phi$ and $\dot{\phi}$. As the geometry specified by ${\tilde g_{\mu\nu}}$ deforms and expands, dark matter undergoes energy transformations. The manner of this energy transfer is highly contingent on our choice of free functions $V(\phi)$, $C(\phi)$, and $D(\phi)$. At a minimum, we need our cosmological model to align with empirical data, which dictates that the dark energy field should approximate a cosmological constant and evolve at a sluggish rate.

We specifically focus on the following functional forms for $V$, $C$, and $D$:
\begin{subequations}
\label{eq:modified_free}
\begin{align}
\label{eq:modified_free:V}
V &= M_V^4 \exp(\beta_V \phi)~, \\
\label{eq:modified_free:C}
C &= C_0 \exp(\beta_C \phi)~, \\
\label{eq:modified_free:D}
D &= M_D^{-4} \exp(\beta_D \phi)~.
\end{align}
\end{subequations}
This represents a natural extension of standard coupled quintessence where $D=0$.

% More analysis and table
In \cref{table:modified_models}, we catalog various models with distinct values for $M_D$, $\beta_C$, and $\beta_D$. Our first primary observation is that the disformal factor can function as an early-time suppressor of the conformal contribution. This insight is crucial since significant conformal couplings are not necessarily at odds with current observational data, provided disformal couplings are present.

\begin{table}
\centering
\begin{tabular}{@{} l l l l l l @{}}
\toprule
\# & Label & $\beta_C$ & $\beta_D$~ & $M_D$ & Temporal Behavior of $x$ \\ \hline
1  & Isolated & 0 & 0 & $\infty$ & Constant \\
2  & Conformal & -0.2 & 0 & $\infty$ & Time-Decreasing \\
3  & Disformal & 0 & 0 & $M_V$ & Time-Increasing \\
4  & Hybrid & -2 & 2 & $M_V$ & Fixed Minimum \\
\bottomrule
\end{tabular}
\caption{Summary of model variants in this study. Model parameters are elaborated in \cref{eq:modified_free}.}
\label{table:modified_models}
\end{table}

% Conclusion
To wrap up, whether conformal or disformal couplings are distinguishable depends on the epoch. While at early times disformal factors generally suppress conformal ones, at later times, they work in conjunction. The key takeaway is that the nature of the coupling can be ambiguous when only cold dark matter is involved.

can you rewrite this (not summarise) and put it in latex code style:

\section{Dynamics of Cosmological Fluctuations}
\label{sec:fluctuations}

We shift our focus to explore the behavior of cosmological fluctuations under our theoretical framework. Initially, we lay down the equations governing these perturbations and then move on to address the implications for cosmological measurements, including variations in the Cosmic Microwave Background (CMB) and the matter power spectrum. Throughout, we will specify the consequences brought about by different coupling scenarios; can these models impart a distinct signature to the spectra due to disformal couplings?

% metric & coordinates
For specificity, we adopt the Newtonian gauge for our calculations. We use $\delta$ exclusively for the matter density contrast, defined as $\delta := \frac{\delta \rho}{\rho}$, while $\delta P$ refers to the pressure fluctuation and $\delta \phi$ to the scalar field fluctuation. A general perturbation operator is represented by $\hat\delta$. The perturbed Einstein-frame metric in this gauge reads as:
\begin{equation}
\label{eq:new_metric}
ds^2 = a^2(\tau)\left[ -(1+2\Psi)d\tau^2 + (1-2\Phi)\delta_{ij}dx^idx^j \right]
\end{equation}
This implies that the trajectories of dark matter particles are governed by the perturbed spacetime metric:
\begin{equation}
\label{eq:new_metric_dis}
d\tilde{s}^2 = Ca^2(\tau)[-(1+2A)\gamma^2d\tau^2
    + 2(\partial_iB)\gamma d\tau dx^i
    + (1-2E)\delta_{ij}dx^idx^j]
\end{equation}
where $A$, $B$, and $E$ depend on both the dark energy background and its perturbations. Their explicit forms are:
\begin{subequations}
\label{eq:new_line}
\begin{align}
A &= \Psi + \frac{\hat{\delta} C}{2C} + \frac{\hat{\delta} \gamma}{\gamma}, \\
B &= \left(\frac{1}{\gamma}-\gamma\right)\frac{\delta \phi}{\phi'}, \\
E &= \Phi - \frac{\hat{\delta} C}{2C}.
\end{align}
\end{subequations}

\section{Conclusions}
In this paper we have studied the observational consequences of an extension to the coupled quintessence scenario, incorporating disformal terms. By keeping dark energy in the slow roll regime, we have focused not on solving the cosmological coincidence problem, but rather on searching for observable signatures of realistic (near $\Lambda$CDM) coupled dark sector theories. Studies like these are an imperative when so little about the dark sector is known and so little can be assumed. 

An important result of our study is that tension between a model with large conformal coupling ($\beta_C$ in our notation) and data can be alleviated by the addition of a disformal interaction. This is because the disformal contribution very effectively suppresses the coupling function $Q$ and it's linear perturbation $\delta Q$ for a significant portion of the Universe's lifetime. The suppression is clearly manifest in both power spectra, as the predictions of the mixed model are very close to those of $\Lambda$CDM, although $\beta_C$ is of order one. We also find that, reformulating the theory in terms of a disformal scalar, the conservation equation for a coupled matter species is solvable, and we have used the solution to derive a condition indicating whether or not a given coupled dark energy model could be interpreted as exhibiting phantom behaviour. 

Our analysis of the perturbations tells us that, as in the standard coupled quintessence model, the disformal term does not affect the gravitational slip. Additionally the growth rate of the matter density contrast and the growth rate of the gravitational potential no longer coincide in models with couplings - we expect this will provide an observational key to breaking degeneracies between information contained in the CMB, gravitational lensing and LSS. We furthermore find that a negative disformal coupling $D$ generically induces dark energy instabilities: perturbations in the scalar field will eventually grow quasi-exponentially.

The results of this paper suggest that it is very difficult to discern between conformal and disformal effects when using only background observables and first order cosmological perturbations (e.g. CMB anisotropies or the matter power spectrum); an analysis of the non-linear regime on small scales it seems will be necessary to look for a `disformal smoking gun'. 

This preliminary study, far from complete, still must make direct contact with data. We leave this task for future work, where we intend to use CLASS's Monte Python to confront the expansive data set open to cosmologists today. It would also be interesting to investigate in how far the mixed model discussed in this paper can be mimicked by a time--varying conformal coupling, such as those studied in \cite{Baldi:2010vv}. Further, more of the theory's functional freedom ($\mathcal{L}_{\rm (DE)}$, $C$, and $D$) must be explored. How robust will our conclusions be under relocations within this function space? In addition, the question of the impact of quantum corrections needs to be addressed. Models with both conformal and disformal couplings between dark matter and dark energy are motivated from string theory (see \cite{Koivisto:2013fta}), and in these models, the scalar field is a DBI field where the functions $C$ and $D$ are specified by the extra--dimensional space. As a consequence, the effective coupling $Q$ has a different form and behaviour. We will turn our attention to such models in future work. 
